# Supplementary material for: LightSeq2: Accelerated Training for Transformer-based Models on GPUs
Source: arXiv:2110.05722 source file (2022-06-16)
Supplement: Supplementary file 1 [file 080appendix.tex]

\subsection{Usage}
